# Supplementary material for: Nematic spin correlations pervading the phase diagram of FeSe$_{1-x}$S$_{x}$
Source: arXiv:2307.08181 source file (2023-07-17)
Supplement: Supplementary file 1 [file RIXS_FeSe1-xSx_SI_2307.pdf]

## Supplemental Material:
## Nematic spin correlations pervading the phase diagram of $FeSe_{1-x}S_x$

Ruixian Liu,[1] Wenliang Zhang,[2] Yuan Wei,[2] Zhen Tao,[1,2] Teguh C. Asmara,[2]
Yi Li,[1] Vladimir N. Strocov,[2] Rong Yu,[3] Qimiao Si,[4] Thorsten Schmitt,[2,*] and Xingye Lu[1,†]

[1]*Center for Advanced Quantum Studies and Department of Physics, Beijing Normal University, Beijing, 100875 P. R. China*
[2]*Photon Science Division, Swiss Light Source, Paul Scherrer Institut, CH-5232 Villigen PSI, Switzerland*
[3]*Department of Physics, Renmin University of China, Beijing 100872, China*
[4]*Department of Physics and Astronomy, Rice Center for Quantum Materials, Rice University, Houston, TX 77005, USA*

### 1. Sample growth and characterization

High-quality $FeSe_{1-x}S_x$ single crystals with self-cleaved edges along the tetragonal $[100]_T$ direction were synthesized using the chemical vapor transport technique with KCl-$AlCl_3$ as the flux [1]. The doping levels are determined with Energy Dispersive Spectroscopy (EDS) and confirmed by resistivity measurements. The typical size of the single crystals is ~1*1*0.1 $mm^3$. Sulfur content $x$ is determined by energy dispersive spectroscopy (EDS) and confirmed by in-plane resistivity measurements (Fig. S1(a)). The short vertical bars in Fig. S1(a) mark the structural transition temperatures ($T_S$). With increasing $x$, $T_S$ is suppressed gradually and finally vanishes at $x \approx 0.17$. In order to determine the nematic quantum critical point (NQCP) accurately, we show in Fig. S1(b) the $T^{1.5}$ dependence of the resistivity curves, which can be well fitted with a linear behavior outside the nematic phase and indicate $x_{QCP} \approx 0.17$ [2]. Therefore, $FeSe_{1-x}S_x$ hosts an electronic nematic state for $x < 0.17$ ($T<T_S$), a NQCP at $x \approx 0.17$, and the tetragonal phase at $x > 0.17$ (and $T>T_S$ for $x \leq 0.17$).

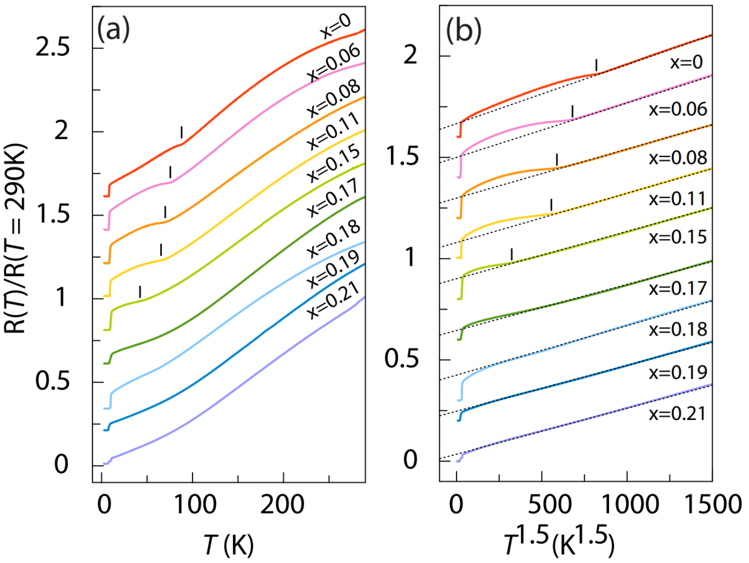


FIG. S1. (a-b) The in-plane resistivity normalized to the data for $T$=290K, measured by a standard four-probe method, as a function of $T$ (temperature) (a) and $T^{1.5}$ (b) for the series of

dopings of $FeSe_{1-x}S_x$ used in this study. The black vertical bars mark the structural transition temperatures. The resistivity curves are shifted vertically for the reason of clarity.

## 2. Characterization of the uniaxial strain

In order to investigate the nematic spin correlations in $FeSe_{1-x}S_x$, we employ a uniaxial-strain device (Fig. S2(c)) to study the spin-excitation anisotropy between $S_h(q_{\|})$ and $S_k(q_{\|})$ [3]. The device is designed based on differential thermal expansion coefficients of an aluminum frame ($\alpha \approx -24\times10^{-6}$/K) and internal invar-alloy ($\alpha \approx -2\times10^{-6}$/K) blocks with a titanium (Ti) sample platform [3]. The Ti platform with a neck in the center bridges the two invar-alloy blocks (Fig. S2). The aluminum, invar alloy, and Ti bridge of the strain device are assembled with epoxy Stycast 2850FT. While cooling, the difference in thermal contraction between the outer aluminum frame and the inner invar-alloy blocks and the Ti platform can generate a sizeable uniaxial strain up to $\varepsilon=\varepsilon_{xx}-\varepsilon_{yy}\approx-0.8\%$ on the neck of the Ti bridge. Such a uniaxial strain can be transferred to the $FeSe_{1-x}S_x$ single crystal glued on the Ti bridge via epoxy Stycast 1266 or Stycast 2850FT. The uniaxial strain of the Ti bridge and $FeSe_{1-x}S_x$ single crystal can be accurately characterized by tracking the relative displacements of some specific spots on the platform and the sample using a microscope camera system [4], for which the sample is loaded in a continuous-flow helium cryostat with an optical window (Janis ST500). Note that the strain characterization can only be performed after the RIXS experiment. Thus, this could result in underestimating the uniaxial strain as the warming-cooling cycling could relax the strain a little bit. We found in our tests that the uniaxial strain changed not much (<20%) after several warming-cooling cycles.

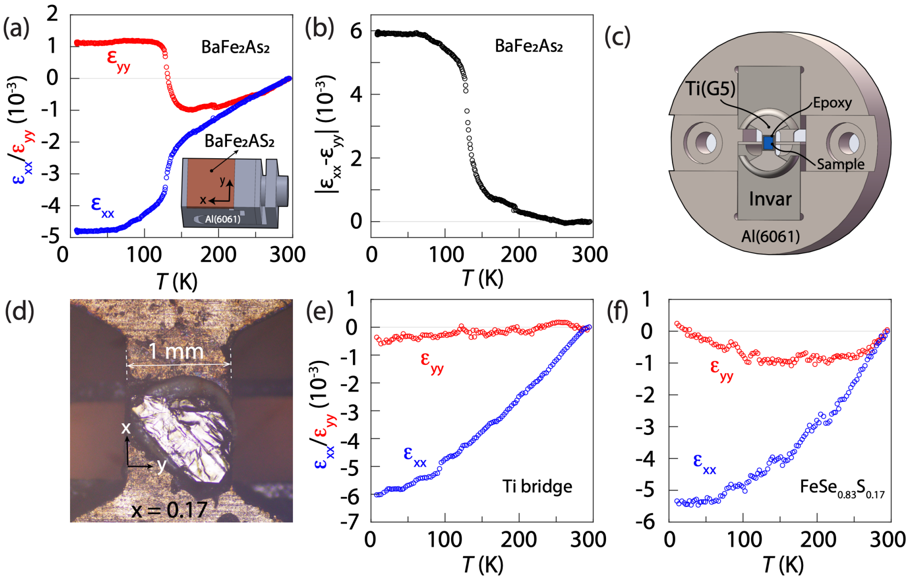


FIG. S2. (a) Anisotropic strain measured on the surface of a uniaxial-pressure detwinned $BaFe_2As_2$ single crystal. The inset shows a mechanical uniaxial-pressure device driven by a

screw and a spring washer. (b) The uniaxial strain of $BaFe_2As_2$ defined as $\varepsilon=\varepsilon_{xx}-\varepsilon_{yy}$. As the orthorhombic lattice distortion is defined as $\delta=(a-b)/(a+b)$, we have $\varepsilon\approx-2\delta$ for the orthorhombic state of a detwinned sample. (c) Schematic of the uniaxial-strain device based on differential thermal expansions between the aluminum frame and the inner invar-alloy blocks. (d) Optical micrograph of the $FeSe_{0.83}S_{0.17}$ single crystal glued on a titanium platform, taken after RIXS measurements. (e), (f) The uniaxial strains measured on the neck of the Ti platform (e) and the $FeSe_{0.83}S_{0.17}$ single crystal (f).

We first characterized the uniaxial strain (orthorhombic lattice distortion) on a $BaFe_2As_2$ single crystal detwinned by a uniaxial-pressure detwinning device (the inset of Fig. S2(a)). Installing the device in the helium cryostat ST500, we can take a series of photos with a microscope during cooling. Employing the Digital Image Correlation Engine (DICe) software [4], we can track the relative displacement of features on the surface of the sample while cooling. The measured strains $\varepsilon_{xx}=(b-b_0)/b_0$, $\varepsilon_{yy}=(a-a_0)/a_0$ of detwinned $BaFe_2As_2$ along x (*b* axis) and y (*a* axis) directions are shown in Fig. S2(a). As the orthorhombic lattice distortion is defined as $\delta=(a-b)/(a+b)$, we have $\varepsilon=\varepsilon_{xx}-\varepsilon_{yy}\approx-2\delta$. The measured $\varepsilon$ in Fig. S2(b) ($\varepsilon=\varepsilon_{xx}-\varepsilon_{yy}\approx-0.6\%$) is indeed consistent with the orthorhombic lattice distortion ($\delta=0.36\%$ at $T<<T_S\approx138$K) of uniaxial-pressured-detwinned $BaFe_2As_2$ measured by high-resolution neutron and x-ray diffraction measurements [5]. This demonstrates that the optical micrograph method is effective in determining the uniaxial strain of samples. Note that the uniaxial strain of $BaFe_2As_2$ at $T$=300K was set to zero. It should be ~0.05% under a typical uniaxial pressure (~20MPa) [5].

For the RIXS measurements, $FeSe_{1-x}S_x$ samples were cleaved in situ in ultrahigh vacuum at based temperature ($T$ = 15 ~ 20 K) [6]. Figure S2(d) shows an optical micrograph of a $FeSe_{0.83}S_{0.17}$ single crystal taken after a RIXS experiment. Using the same method, we measured the uniaxial strain on the surface of the sample and Ti platform. Figure S2(e) and S2(f) show the characterization of the uniaxial strain measured on the Ti platform (Fig. 2(e)) and the $FeSe_{0.83}S_{0.17}$ crystal (Fig. S2(f)) as shown in Fig. S2(d). The calculated uniaxial strain is $\varepsilon=\varepsilon_{xx}-\varepsilon_{yy}\approx-0.6\%$.

## 3. Additional RIXS spectra of strained and unstrained $FeSe_{1-x}S_x$

For the RIXS measurements, all the spectra were collected with $\pi$ polarization. We define the momentum transfer **q** in reciprocal space as $\mathbf{q} = H\mathbf{a}^* + K\mathbf{b}^* + L\mathbf{c}^*$, where $H, K, L$ are Miller indices and $\mathbf{a}^* = \mathbf{e}_a 2\pi/a$, $\mathbf{b}^* = \mathbf{e}_b 2\pi/b$, and $\mathbf{c}^* = \mathbf{e}_c 2\pi/c$ are reciprocal lattice unit (r.l.u.) vectors with $a \approx 5.3$ Å, $b \approx 5.3$ Å and $c \approx 5.5$ Å. All spectra in this paper are normalized to the integrated intensity of the fluorescence signal in the energy loss range of 1 ~ 10 eV. Figure S3(a) and Figure S3(c) show the momentum-dependent RIXS spectra of unstrained $FeSe_{1-x}S_x$ samples ($x$ = 0.08, 0.18) with momentum transfer along $H$ direction at $T$ = 15K. Figure S3(b) shows RIXS spectra of uniaxial-strained $FeSe_{0.89}S_{0.11}$ ($x$ = 0.11) at $T$ = 15K and 100K along $H$ and $K$ direction,

measured at Fe $L_3$-edge. The spin-excitation anisotropy gradually decreases at a higher temperature. Magnetic excitation spectra along [*H, H*] direction in $FeSe_{0.94}S_{0.06}$ and $FeSe_{0.81}S_{0.19}$ at $T = 20$K are shown in Figure S3(d-e). Dispersive magnetic excitations are observed as a broad peak in the low-energy region. With increasing momentum transfer $q_{\|}$ the energy position of the magnetic excitations shift away from the elastic peak and the intensity increases.

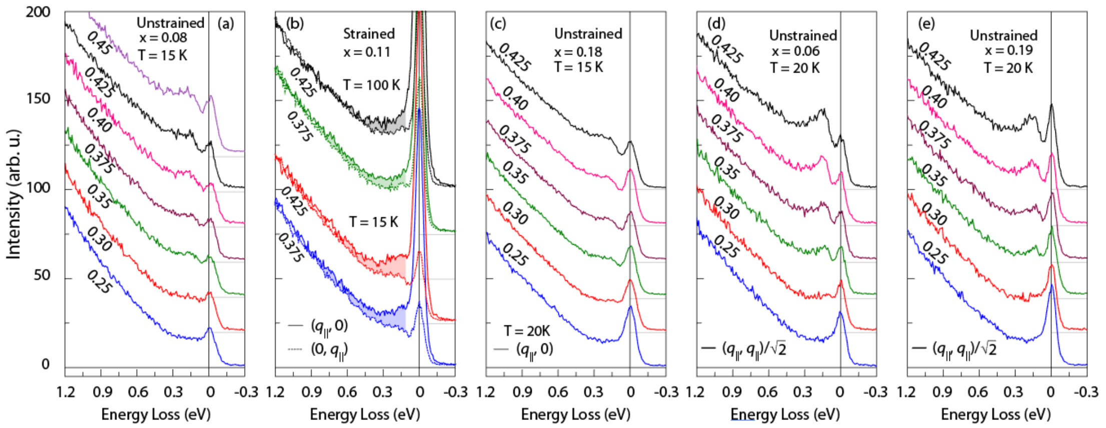


FIG. S3. Momentum-dependent RIXS spectra measured on unstrained ($x = 0.08$, 0.18, 0.06 and 0.19) and uniaxial-strained ($x = 0.11$) $FeSe_{1-x}S_x$ samples. (a), (c) $q_{\|}$-dependent RIXS spectra along H direction of unstrained x = 0.08 and 0.18 samples at $T = 15$ K. (b) RIXS spectra along H (solid curves) and K (dashed curves) directions of uniaxial-strained x = 0.11 sample at $T = 15$ and 100K. The colored areas mark the difference between $I_h(q_{\|})$ and $I_k(q_{\|})$. (d), (e) RIXS spectra along [*H, H*] directions of unstrained $x = 0.06$ and 0.19 samples at $T = 20$K.

## 4. Fitting of the RIXS spectra of uniaxial-strained $FeSe_{0.83}S_{0.17}$

In order to quantitatively analyze all RIXS spectra, we employ an energy resolution-limited Gaussian function, a quadratic polynomial, and a general damped harmonic oscillator function to fit elastic peak scattering ($I_{el}$), fluorescence background ($I_{fluo}$(E)), and magnetic excitation ($S(E)$), respectively [6, 7].

The RIXS spectrum is expressed as:

$$I(E) = I_{fluo}(E) + S(E) + I_{el}(E) \qquad (1)$$

The elastic peak (Gaussian functions) is described by:

$$I_{el} = a_0 \exp\left(-\ln(2) * \frac{(x-x_0)^2}{dx^2}\right) \qquad (2)$$

where $x_0$ is the center of the elastic peak.

For fluorescence in iron-based superconductors (FeSC) can be captured by (quadratic polynomial functions),

$$I_{fluo} = (bE^2 + aE) \cdot (1 - g_\gamma) + I_0 \exp(-\alpha E) \cdot\ g_\gamma + G \qquad (3)$$

with

$$g_\gamma = (\exp\left(\frac{E+E^*}{\Gamma}\right) + 1)^{-1} \qquad (4)$$

$$G = A_0 \exp\left(\frac{(E+E_S)^2}{2\sigma^2}\right) \qquad (5)$$

where $G$ is a Gaussian function

The first and second term of formula (3) describe the low energy loss with second-order polynomial behavior and high-energy loss with exponential behavior of the fluorescence line, respectively. $g_\gamma$ generates a smooth connection between these two behaviors.

The damped magnetic excitation in FeSC (damped harmonic oscillator function) is described as:

$$S(q, E) = A \frac{E_0}{1-e^{-\beta E}} \frac{2\gamma E}{\left(E^2-{E_0}^2\right)^2+(E\gamma)^2} \qquad (6)$$

$\beta = \frac{1}{k_B T}$ ($k_B$ is Boltzmann constant).

where $E_0$ is the underdamped energy and $\gamma$ describes the excitation lifetime (the damping rate).

Figure S4 (a-f) show the fitting of the RIXS spectra $I_h(q_{\|})$ and $I_k(q_{\|})$ for the uniaxial-strained $FeSe_{0.83}S_{0.17}$. The results reveal strong anisotropy between the spin excitations $S_h(q_{\|})$ and $S_k(q_{\|})$ in the whole $q_{\|}$ range measured. RIXS spectra along [$H$, $H$] direction and their fitting are shown in Fig. S4 (g-l). All spectra are collected at $T$ = 20 K and the fitting results are shown and discussed in the main text.

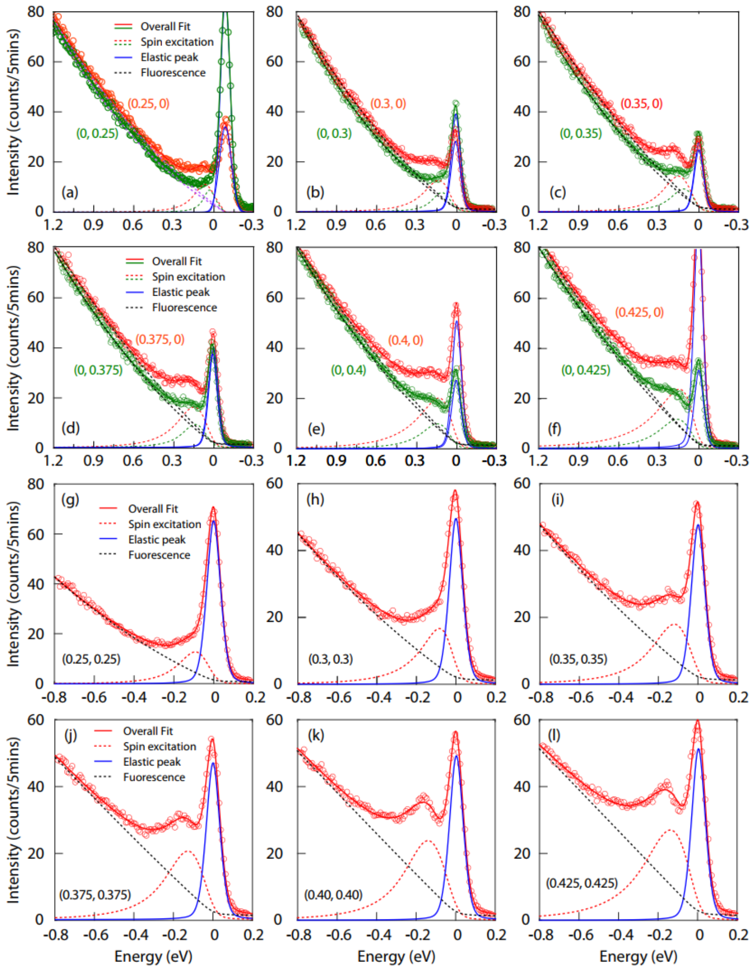


FIG. S4. Fitting of the RIXS spectra for uniaxial-strained $x$=0.17, measured at $T$ = 20 K. (a-f) RIXS spectra along [$H$, 0] (red open circles) and [0, $K$] (green open circles) directions. (g-l) RIXS spectra along [$H$, $H$] (red open circles) direction, which is not affected by uniaxial strain. The red and green dashed curves, black dashed curves, and solid blue curves are fitting components of spin excitations, fluorescence contribution, and the elastic peak, respectively. The red and green solid curves represent the overall fitting of the RIXS spectra.

**Reference:**


[1] D. Chareev *et al.*, Single crystal growth and characterization of tetragonal $FeSe_{1-x}$ superconductors. CrystEngComm, **15**, 1989-1993 (2013).

[2] M. Bristow *et al.* Anomalous high-magnetic field electronic state of the nematic superconductors $FeSe_{1-x}S_x$. Phys. Rev. Research. **2**, 013309 (2020).

[3] V. Sunko et al., Direct observation of a uniaxial stress-driven Lifshitz transition in Sr2 RuO4 . npj Quantum Materials **4**, 46 (2019).

[4] B. Pan *et al.* Two-dimensional digital image correlation for in-plane displacement and strain measurement: a review. Meas. Sci. Technol. **20**, 0620001 (2009).

[5] X. Lu *et al.*, Impact of uniaxial pressure on structural and magnetic phase transitions in

electron-doped iron pnictides. Phys. Rev. B **93**, 134519 (2016).
[6] X. Lu *et al*. Spin-excitation anisotropy in the nematic state of detwinned FeSe. Nat. Phys. **18**, 806-812 (2022).
[7] J. Pelliciari *et al*., Reciprocity between local moments and collective magnetic excitations in the phase diagram of $BaFe_2(As_{1-x}P_x)_2$. Commun Phys. **2**, 139 (2019).
